# Supplementary material for: Exemplar-based Pattern Synthesis with Implicit Periodic Field Network
Source: arXiv:2204.01671 source file (2022-04-15)
Supplement: Supplementary file 1 [file draft_supp.tex]

\documentclass[final]{cvpr}

\newcommand{\final}{0}

%\input{paper}
\input{supp.tex}
